# Supplementary material for: Sim2real gap is non-monotonic with robot complexity for morphology-in-the-loop flapping wing design
Source: arXiv:1910.13790 source file (2019-10-30)
Supplement: Supplementary file 1 [file 99_appendix.tex]

\section*{Supplementary Data} 

This supplementary provides additional details on the simulation, manufacture and evolutionary design tools.  Simulation and design tools and sim2real results are provided in supplied source code and data hosted at \textbf{$<$location to be advised for CoRL2019$>$}.

\subsection*{Simulator}

Software for the flapping wing morphology simulator is provided in the software under the simulation directory.

The simulation of the flapping wing is configured as a set of finite element "blades" that are connected to each other by elastic rotational spring physics elements.  As a result, shape, span, elasticity and inertia can be discretised along the wing.

%The aerodynamics used for each blade element is an implementation of the quasistatic model for flapping wing from  \textit{et al.} \cite{sane2002aerodynamic}.  That study considered a flat, rigid, scaled version of the wing of an insect, and experimentally produced a model of time domain forces for quasi static flapping as the sum of inertial, translational, rotational and wake capture forces.

%For a given wing, blade element analysis can be used to predict translational  forces solving lift and drag of the total wing as the sum of the forces on the set of chordwise aligned wing blades.  This approach has been used in evolutionary design of ornithopter morphology previously in \cite{shim2006evolving} although that example did not include the rotational part of the quasi-static model nor were the results transferred to reality.

For our aerodynamic simulation, we modelled our flapping wing design as a set of spanwise aligned connected flat blade elements. Rigid thin flat plates are often used to model simple aerodynamic wings they have well characterised aerodynamic coefficients at a wide variety of Reynolds numbers and across the full sweep of angle of attack \cite{sheldahl1981aerodynamic}. To implement our blade element quasi static model for an individual flat plate we utilised that data to produce translational forces, while rotational forces were modelled directly inline with the quasi-static model put forward by Sane \textit{et al.} \cite{sane2002aerodynamic}.  Wake capture, which is the effect of the wing interacting with the wake it has created in its previous stroke, is a poorly described force to date and we have not included it as a simulation component.

Our quasi-static blade element aerodynamics was incorporated as an extension into an open source robotics simulator, PYROSIM \cite{kriegman2017simulating}. Quasi-static forces were produced for all flat plates within a simulation, while the underlying physics simulator resolved the inertial and elastic response of the wing.  This approach has been used in evolutionary design of ornithopter morphology previously in \cite{shim2006evolving} although that example did not include the rotational part of the quasi-static model nor were the results transferred to reality.

A full wing is constructed in the simulator as shown in Figure \ref{fig:exampleWingSequence}(a) of the main article. The wing is comprised of a set of flat plate blades each with their own geometry, aligned along the spanwise direction of the wing and together defines the overall shape and  span of the wing.  The blades are connected by rotational spring joints to allow  both chordwise twisting and spanwise bending elastic deformations when the wing was under load. \RSSFIXME{As discussed previously, morphological shape, size and stiffness are known to be important for natural fliers \cite{li2017wing} and are therefore made available for selection within our bio-inspired parameterised design morphospace.}

\subsection*{Manufacture data}

Materials used in the construction are listed in Table \ref{tab:wingMaterials}. 

The breakdown of manufacturing times for one wing is shown in Table~\ref{tab:manuTimeBreakdown}.

\begin{table}[H]
%\begin{table}{r}{0.6\textwidth}
\begin{center}
\caption{List of materials used in wing manufacture}
\label{tab:wingMaterials}
\begin{tabular}{|c|c|c|}
\hline
Material & Component & Specification  \\
\hline
Carbon Rod  & spar / rib stiffeners & 0.8mm and 0.4mm diameter \\
Stainless steel wire & rib spring & 0.1mm, 0.13mm, 0.17mm  \\
Aluminised Mylar & skin & 5$\mu$m \\
ABS plastic & wing root mount  & 3D printed design \\
\hline
\end{tabular} 
\end{center}
\end{table}
%\end{table}

\begin{table}[H]
%\begin{wraptable}{r}{0.6\textwidth}
\caption{Manufacturing time breakdown for one wing}
\label{tab:manuTimeBreakdown}
\centering  
\begin{tabular}{|c|c|}
\hline
Activity     &  Time\\
\hline
3D Printing wing roots     & 15 min\\
Solvent bath      &  1 day (waiting time)\\
Producing wing template      & 15 min\\
Manufacturing wing structure      & 30 min\\
Epoxy curing time      & 1 day (waiting time)\\
Manufacture wing skin    & 30 min\\
Wing assembly       & 30 min\\
\hline
\end{tabular}
%\end{wraptable}
\end{table}

\subsubsection*{Flapping Wing Test Rig}

We assessed real world performance of manufactured wings using a flapping wing test rig as depicted with a mounted wing in Figure \ref{fig:exampleWingSequence}(e). Our test rig drives the wing repeatedly through a single flapping axis using a linear solenoid actuator with magnetic plungers similar to the design demonstrated by Kok \textit{et al}.~\cite{kok2016design}. Position feedback was provided by a laser displacement sensor (Keyence IL100) that measured the position of the magnetic plunger which defined angular position of the wing. An Arduino Due \cite{arduino} measured the position feedback and commanded the actuator such that real time angular position of wing stroke could be accurately controlled. The actuator and wing assembly was mounted on an ATI Nano17 Force/Torque transducer such that forces generated by the actuated wing were recorded by a National Instruments data acquisition system \cite{niusb6003} at a sampling frequency of 100kHz. The flapping test rig was capable of producing controlled oscillation beyond 10Hz dependant on the specific wing attached over a angular range of $\pm40^o$.  This study set a fixed sinusoidal pattern at 5Hz to facilitate arbitrary  morphology-in-the-loop design without risking damage to either the wing or apparatus.

Measured data from the simulation to reality transfers are provided in the supplied software within the data directory.

\subsection*{Evolutionary design}

Software for the evolutionary design is provided in the software under the evolution directory.

The evolutionary approach included the development of a genotype descriptor that defines any  individual wing, and the evolutionary optimiser that searches for the optimal design.

Our genotype for morphology is defined using Compositional Pattern Producing Networks (CPPNs) \cite{stanley2007compositional}.  A feature of the CPPN that lends itself to evolved robotic design is that its structure provides scope for a range of observed characteristics seen in natural genetic expression such as repetition, repetition with variation, symmetry, imperfect symmetry and regularity which are not easily reproduced using direct encoded genotypes.  CPPNs are structured similarly to an artificial neural networks using edges and  nodes that accumulate their weighted inputs but each node is also allocated an activation function which operates on the incoming accumulated signal to produce the node output.  The operator function set for hidden nodes in our design included sinusoid, absolute, negative, absolute, square and square root of absolute, while all output nodes applied the sigmoid function to normalise the output space.  This choice of operators provided scope for repetition, and symmetry with and without variation.

The morphology CPPN was expressed using a genotype contained morphology expression array. The number of blades in a simulation wing (or ribs in the real wing) was defined by the length of the morphology expression array and each entry in that array includes values specifying the position of the blade relative to its inboard neighbour and a "similarity" value. Similarity values were defined to be between 0 and 1, while the relative position of a blade was limited to between 30mm and 150mm.  The length of the wing was defined as the sum of each blade elements position value.  This morphology expression array has variable length and we added functionality within the genotype to allow the addition and removal of entries in the array at any location as a means of mutation. When we express the morphology CPPN using the input values from the expression array, the CPPN outputs "paint" the wing by defining for each blade its chord length (distance from leading edge to trailing edge) and its elastic characteristics in chordwise and spanwise directions.   

%Evolution on a population of genotypes is enabled by producing offspring from the existing population.  In our genotype,  both the controller and morphology expression arrays and their CPPNs could be mutated from existing population members and/or  crossed-over with other individuals to form new descendants.  Mutations could adjust length and values of expression arrays and alter the CPPNs through adding, removing and changing nodes and edges.

% Genotype expression also defined the physical phenotype for manufacture and test using our defined method.  The  connection from simulation wing to physical evaluation is diagrammatically shown in figure \ref{fig:exampleWingSequence}(a)-(d) which shows a simulated wing converted automatically to a manufacture blueprint which can be fabricated and then tested.   We defined a mapping from simulation phenotype to real wing using the simple rules to facilitate automation and they define structure of a physical wing as a set of flexible ribs placed along a spar and a skin attached trimmed to the piece-wise linear outline of the ribs to remove unsupported material.  The specification for wing span, the number of ribs and their location, elasticity and chord dimension are determined from the genotype, resulting in a physical wing with similar parameters to that of the simulation phenotype. 

In this study we the multi-objective Non-dominated Sorting Genetic Algorithm II (NSGA-II) \cite{deb2002fast}  evolutionary optimisation methods to search for individuals using four objective dimensions defined in Table \ref{tab:evolutionaryDesignSettings}.  

When optimising across more than one dimension, rather than determining a single best morphology, the NSGA-II algorithm produces a set (known as a front) of non-dominated individuals.  Each individual represents one distinct design that is superior to all the others in the population on at least one objective.  Multi-objective optimisation is commonly used to maintain a diverse set of high performance designs.

\begin{table}
%\begin{wraptable}{r}{0.5\textwidth}
\centering  
\caption{Evolutionary Design Settings}
\begin{tabular}{|c|c|}
\hline
Setting     &  Value\\
\hline
Algorithm     & NSGA-II\\
Objective 1      & Lift \\
Objective 2      & Power or Torque \\
Objective 3      & Feasibility Distance \\
Objective 4      & Age \\
Population Size $\mu$    & 100\\
Generations       & 200\\
Probability Crossover     & 0.2\\
Probability Mutation      & 0.8\\
Upper limit for Lift & 0.2N \\
Evaluation period & 2seconds\\
\hline
\end{tabular}
\label{tab:evolutionaryDesignSettings}
\end{table}
%\end{wraptable}

Our first two objectives drove the population towards high performance systems by increasing the amount of lift produced and reducing the amount of drive requirement (power and torque) required to achieve it.  The remaining two objectives were included only to improve the robustness of the evolution but played no result in final analysis.  

Objective 3 is a penalty measure of "distance" in the phenotypic space for any wing that cannot be manufactured (for instance a specification may include unrealisable dimensions) to the nearest feasible wing design. This measure reduced to zero within only a few generations ensuring that the population evolves individuals with valid chord length, span and elasticity.  

Objective 4 is the age of each individual using the definition put forward in Age Fitness Pareto Optimisation \cite{schmidt2011age}. Using age as an evolutionary objective has been shown to promote diversity and reduce premature convergence to non-optimal solutions during evolution, however all ages are set to zero at the end of the evolution when determining the final non-dominated front. 

To provide additional constraints on the evolved designs, the simulated lift was clamped at a minimum value of 1gram (10mN) and maximum value of 20grams (200mN) which is a reasonable upper limit for search given that biological examples are typically weigh less than 10grams.

\subsection*{Sim2real data}

Data files for transferred wing designs, simulation and test rig results are included in the results directory.

% \RSSFIXME{Figure \ref{fig:results_EVC} shows the cyclical time domain response of the best transferred wing, EV-C, in both simulation and reality.  The plot shows the range of lift (shaded) with time during a forward stroke and backstroke of the sinusoidal control input.  EV-C is an example of reality outperforming the predicted simulation performance and results in a positive $STR$. While our driver for our  research program is automating the ability to cross the reality gap, we not that the simulation has reasonably characterised peak lift in the forward and back strokes (time 0.05s and 0.12s) but has not accurately predicted the maintained lift during the transition between forward and backstroke (time 0.075-0.1s).  This period is associated with wake capture as the wing interacts with the displaced airflow from the previous stroke and is not included in our simulation model. }

% \begin{wrapfigure}{R}{.9\textwidth}
%   \centering
%     \includegraphics[trim=0 3.5in 0 .8cm,clip,width=0.9\textwidth] {images/BLP_NDF60_lift_clean.png}
%     \includegraphics[trim=0 3.3in 0 .8cm,clip,width=0.9\textwidth] {images/BLP_NDF60_testrigWaveform.png}
%   \caption{Lift vs time repeatability for EV-C wing in  simulation (top) and reality (bottom).  }
%   \label{fig:results_EVC}
% \end{wrapfigure}
